# Supplementary material for: Unraveling time-varying causal effects of multiple exposures: integrating Functional Data Analysis with Multivariable Mendelian Randomization
Source: arXiv:2512.19064 source file (2026-11-16)
Supplement: Supplementary file 1 [file MV_FMR_Supp_Mat.pdf]

# Unraveling time-varying causal effects of multiple exposures: integrating Functional Data Analysis with Multivariable Mendelian Randomization

## Supplementary Material

Nicole Fontana, Francesca Ieva, Luisa Zuccolo, Emanuele Di Angelantonio, Piercesare Secchi

**Supplementary Method 1:** Functional Principal Component Analysis with PACE method

**Supplementary Table 1:** Coverage rate of the comparison of MV-FMR and U-FMR across simulation scenarios 1–3

**Supplementary Table 2:** Conditional F-statistics of the comparison of MV-FMR and U-FMR across simulation scenarios 1–3

**Supplementary Table 3:** Sensitivity analysis of MV-FMR performance under alternative exposure-outcome models

**Supplementary Table 4:** Sensitivity analysis of MV-FMR performance under different proportions of overlapping instruments and different mediation strengths with a binary outcome.

**Supplementary Table 5:** Sensitivity analysis of MV-FMR performance under varying longitudinal data sparsity with binary outcome

**Supplementary Figure 1:** Mean time-varying causal effect estimates across different exposure-outcome model combinations with a binary outcome

### Supplementary Method 1: Functional Principal Component Analysis with PACE method

Functional Principal Component Analysis (FPCA) provides a low-dimensional representation of smooth functional data. For each exposure  $X_j(t)$  observed over  $t \in [0, T]$ , let  $\mu_j(t)$  denote the mean trajectory and  $\text{cov}(X_j(s), X_j(t))$  the covariance function. The eigendecomposition of the covariance operator yields:

$$\text{cov}(X_j(s), X_j(t)) = \sum_{k=1}^{\infty} \lambda_{j,k} \phi_{j,k}(s) \phi_{j,k}(t), \quad (\text{S1})$$

where  $\lambda_{j,1} \geq \lambda_{j,2} \geq \dots \geq 0$  are the eigenvalues and  $\phi_{j,k}(t)$  are the orthonormal eigenfunctions. By the Karhunen-Loève theorem, each individual trajectory can be written as:

$$X_j(t) = \mu_j(t) + \sum_{k=1}^{\infty} \xi_{j,k} \phi_{j,k}(t), \quad (\text{S2})$$

where  $\xi_{j,k} = \int_0^T (X_j(t) - \mu_j(t)) \phi_{j,k}(t) dt$  are uncorrelated scores with variance  $\text{var}(\xi_{j,k}) = \lambda_{j,k}$  and  $\text{cov}(\xi_{j,k_1}, \xi_{j,k_2}) = 0$  for  $k_1 \neq k_2$ .

In practice, longitudinal data are often sparse and irregularly sampled. To address this, we implement the Principal Analysis by Conditional Estimation (PACE) method [? ], modeling observed measurements as  $X_{j,i}(t_{j,i,l}) = X_j^*(t_{j,i,l}) + \epsilon_{j,i,l}$  with  $\epsilon_{j,i,l} \sim \mathcal{N}(0, \sigma_j^2)$ , where  $X_j^*(t)$  is the true underlying trajectory and  $\epsilon_{j,i,l} \stackrel{\text{iid}}{\sim} \mathcal{N}(0, \sigma_j^2)$  represents measurement error. Under the assumption that individual trajectories follow the FPCA representation above, the principal component scores are estimated via conditional expectation.

$$\hat{\xi}_{j,k} = \mathbb{E}[\xi_{j,k} | \mathbf{X}_j] = \lambda_{j,k} \boldsymbol{\phi}_{j,k}^T \boldsymbol{\Sigma}_j^{-1} (\mathbf{X}_j - \boldsymbol{\mu}_j). \quad (\text{S3})$$

The expansion Eq. (S2) is truncated at  $K_j$  components, with  $K_j$  selected automatically via cross-validation (see Section 2.3.2 in the main manuscript).

**Supplementary Table 1: Coverage rate of the comparison of MV-FMR and U-FMR across simulation scenarios 1–3**

| Scenario | Continuous Outcome |               | Binary Outcome |               |
|----------|--------------------|---------------|----------------|---------------|
|          | MV-FMR             | U-FMR         | MV-FMR         | U-FMR         |
| 1        | 0.545 (0.277)      | 0.621 (0.278) | 0.279 (0.230)  | 0.024 (0.029) |
|          | 0.560 (0.275)      | 0.697 (0.246) | 0.279 (0.249)  | 0.027 (0.035) |
| 2        | 0.296 (0.192)      | 0.207 (0.186) | 0.523 (0.320)  | 0.201 (0.202) |
|          | 0.979 (0.115)      | 0.674 (0.284) | 1.000 (0.000)  | 0.695 (0.357) |
| 3        | 0.549 (0.269)      | 0.417 (0.259) | 0.181 (0.158)  | 0.020 (0.019) |
|          | 0.608 (0.259)      | 0.522 (0.249) | 0.176 (0.165)  | 0.021 (0.018) |

**Table S1.** Performance comparison of MV-FMR and U-FMR across simulation Scenarios 1–3, for continuous and binary outcomes. Values are presented as mean (SD) of the pointwise 95% coverage rate for  $\beta_1(t)$  (first line) and  $\beta_2(t)$  (second line).

**Supplementary Table 2: Conditional F-statistics of the comparison of MV-FMR and U-FMR across simulation scenarios 1–3**

| Scenario | $X_1$ (cFF) |             |             | $X_2$ (cFF) |             |             |
|----------|-------------|-------------|-------------|-------------|-------------|-------------|
|          | PC1         | PC2         | PC3         | PC1         | PC2         | PC3         |
| 1        | 8.45 (1.14) | 6.49 (0.85) | 1.74 (0.25) | 8.35 (1.05) | 6.49 (0.88) | 1.74 (0.23) |
| 2        | 8.45 (1.14) | 6.49 (0.85) | 1.74 (0.25) | 8.35 (1.05) | 6.49 (0.88) | 1.74 (0.23) |
| 3        | 8.48 (1.16) | 6.46 (0.82) | 1.76 (0.24) | 5.49 (0.65) | 4.33 (0.70) | 1.51 (0.21) |

**Table S2.** Conditional F-statistics (mean (SD)) for each principal component (PC1–PC3) across the three simulation scenarios. Results are reported separately for Exposure 1 (cFF) and Exposure 2 (cFF), and are the same for both continuous and binary outcome. PC1, PC2, and PC3 denote the first, second, and third principal components, respectively.

**Supplementary Table 3: Sensitivity analysis of MV-FMR performance under alternative exposure-outcome models**

Table S3.1 summarizes the functional forms of the exposure-outcome relationships used in additional simulation analyses for Scenarios 1 and 3. Each row represents specific combination of true time-varying effects  $\beta_1(t)$  and  $\beta_2(t)$ , allowing evaluation of MV-FMR performance under alternative functional forms.

| Case | Functions $(\beta_1(t), \beta_2(t))$                           |
|------|----------------------------------------------------------------|
| A    | $(0.4 - 0.02 \cdot t, 0.4 - 0.02 \cdot t)$                     |
| B    | $(0.4 - 0.02 \cdot t, 0.1 \cdot \mathbf{1}(t < 20))$           |
| C    | $(0.1 \cdot \mathbf{1}(t < 20), 0.4 - 0.02 \cdot t)$           |
| D    | $(0.1 \cdot \mathbf{1}(t < 20), 0.1 \cdot \mathbf{1}(t < 20))$ |

**Table S3.1.** Functional forms of the exposure-outcome relationships used in additional simulation analyses for Scenarios 1 and 3. Each case specifies the true time-varying effects  $\beta_1(t)$  and  $\beta_2(t)$  considered to evaluate the robustness of MV-FMR under alternative functional forms.

| Scenario | Case | Method | ISE $\beta_1$ | Coverage $\beta_1$ | ISE $\beta_2$ | Coverage $\beta_2$ |
|----------|------|--------|---------------|--------------------|---------------|--------------------|
| 1        | A    | MV-FMR | 0.006 (0.004) | 0.363 (0.216)      | 0.005 (0.002) | 0.381 (0.232)      |
|          |      | U-FMR  | 0.026 (0.042) | 0.382 (0.287)      | 0.021 (0.033) | 0.448 (0.277)      |
|          | B    | MV-FMR | 0.005 (0.002) | 0.358 (0.157)      | 0.001 (0.001) | 0.825 (0.196)      |
|          |      | U-FMR  | 0.007 (0.003) | 0.135 (0.180)      | 0.016 (0.032) | 0.691 (0.234)      |
|          | C    | MV-FMR | 0.001 (0.001) | 0.801 (0.210)      | 0.005 (0.002) | 0.351 (0.160)      |
|          |      | U-FMR  | 0.019 (0.041) | 0.604 (0.281)      | 0.007 (0.002) | 0.146 (0.176)      |
|          | D    | MV-FMR | 0.001 (0.000) | 0.571 (0.144)      | 0.001 (0.000) | 0.591 (0.151)      |
|          |      | U-FMR  | 0.002 (0.001) | 0.274 (0.216)      | 0.002 (0.002) | 0.260 (0.209)      |
| 3        | A    | MV-FMR | 0.006 (0.003) | 0.401 (0.163)      | 0.004 (0.001) | 0.467 (0.179)      |
|          |      | U-FMR  | 0.053 (0.039) | 0.234 (0.216)      | 0.013 (0.012) | 0.347 (0.239)      |
|          | B    | MV-FMR | 0.006 (0.003) | 0.353 (0.106)      | 0.001 (0.000) | 0.842 (0.143)      |
|          |      | U-FMR  | 0.010 (0.003) | 0.170 (0.190)      | 0.008 (0.015) | 0.532 (0.249)      |
|          | C    | MV-FMR | 0.001 (0.001) | 0.771 (0.193)      | 0.004 (0.002) | 0.390 (0.133)      |
|          |      | U-FMR  | 0.037 (0.037) | 0.355 (0.264)      | 0.006 (0.002) | 0.187 (0.186)      |
|          | D    | MV-FMR | 0.001 (0.001) | 0.507 (0.153)      | 0.001 (0.000) | 0.585 (0.133)      |
|          |      | U-FMR  | 0.003 (0.001) | 0.175 (0.228)      | 0.001 (0.000) | 0.271 (0.211)      |

**Table S3.2.** Sensitivity analysis of MV-FMR performance under different functional forms of the exposure-outcome relationships. Values are mean (SD) of the ISE and pointwise 95% coverage rate for estimated  $\beta_1(t)$  and  $\beta_2(t)$  with continuous outcome in Scenarios 1 and 3. Cases A–D correspond to the function definitions in Table S3.1.

**Supplementary Table 4: Sensitivity analysis of MV-FMR performance under different proportions of overlapping instruments and different mediation strengths with a binary outcome.**

| Scenario 1 |               |               |               |               |
|------------|---------------|---------------|---------------|---------------|
| $p_{12}$   | 0.15          | 0.30          | 0.50          | 0.80          |
|            | 0.035 (0.009) | 0.034 (0.010) | 0.034 (0.010) | 0.035 (0.010) |
|            | 0.033 (0.011) | 0.033 (0.011) | 0.034 (0.010) | 0.033 (0.010) |
| Scenario 3 |               |               |               |               |
| $\gamma$   | 0.15          | 0.30          | 0.50          | 0.80          |
|            | 0.039 (0.011) | 0.039 (0.010) | 0.044 (0.012) | 0.044 (0.012) |
|            | 0.054 (0.012) | 0.054 (0.012) | 0.070 (0.014) | 0.069 (0.012) |

**Table S4.** MV-FMR performance under varying proportions of overlapping variants (Scenario 1) and different mediation strengths (Scenario 3) for binary outcome. Values are mean (SD) of the ISE for estimated  $\beta_1(t)$  (first line) and  $\beta_2(t)$  (second line) within each cell.

**Supplementary Table 5: Sensitivity analysis of MV-FMR performance under varying longitudinal data sparsity with binary outcome.**

| nSparse    |               |               |               |               |
|------------|---------------|---------------|---------------|---------------|
|            | 5             | 10            | 25            | 50            |
| Scenario 1 | 0.110 (0.015) | 0.035 (0.009) | 0.003 (0.003) | 0.005 (0.012) |
|            | 0.110 (0.015) | 0.034 (0.010) | 0.003 (0.003) | 0.006 (0.010) |
| Scenario 3 | 0.126 (0.017) | 0.044 (0.012) | 0.005 (0.006) | 0.004 (0.007) |
|            | 0.126 (0.019) | 0.044 (0.012) | 0.004 (0.004) | 0.004 (0.007) |

**Table S5.** MV-FMR performance under varying longitudinal data sparsity for binary outcome. Values are mean (SD) of the ISE for estimated  $\beta_1(t)$  (first line) and  $\beta_2(t)$  (second line) at different numbers of observation points per individual (nSparse) in Scenarios 1 and 3.

**Supplementary Figure 1: Mean time-varying causal effect estimates across different exposure-outcome model combinations with a binary outcome**

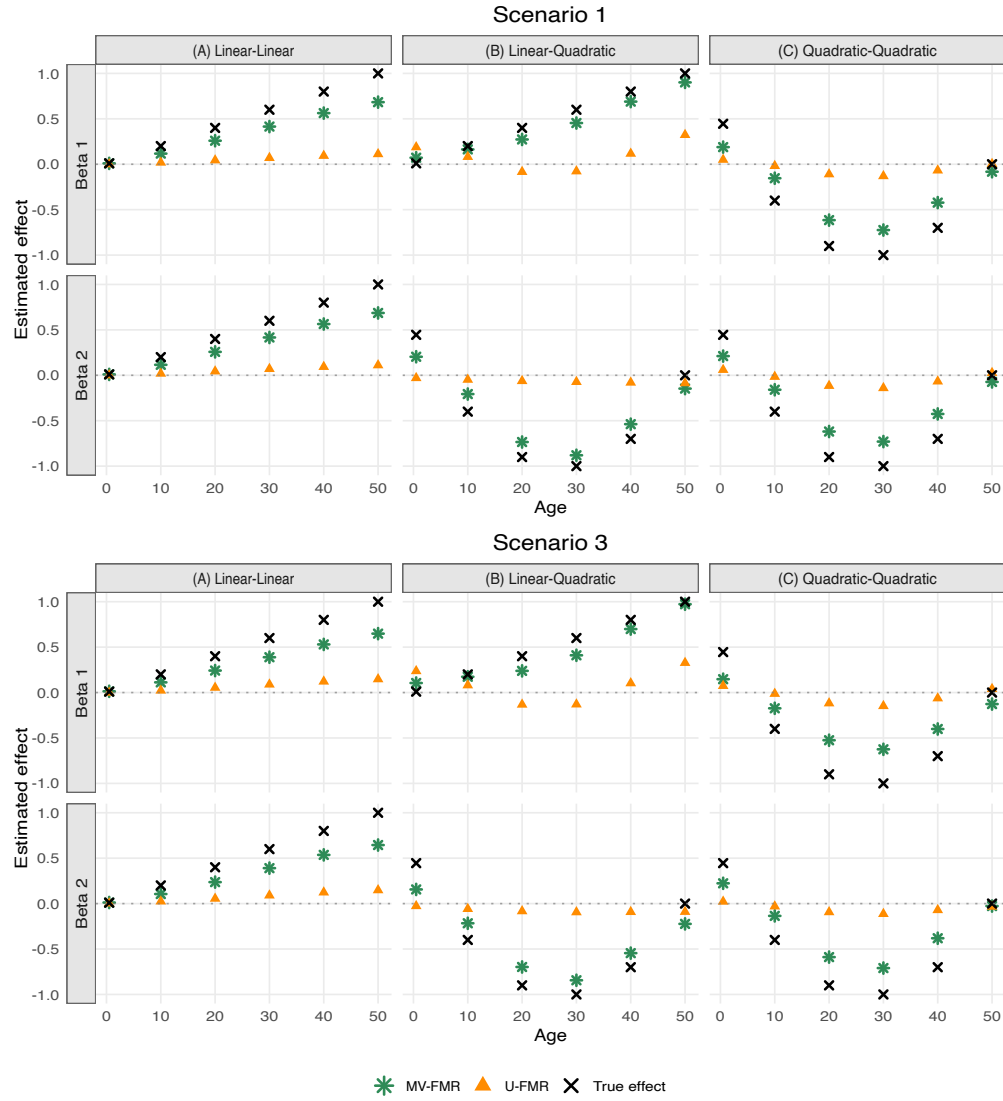

**Fig. S1.** Mean time-varying causal effect estimates at six time points for comparing MV-FMR and U-FMR with binary outcome. Columns represent different exposure-outcome model combinations, rows show  $\beta_1(t)$  and  $\beta_2(t)$ . Black crosses indicate the true causal effects, green stars show MV-FMR estimates, and orange triangles the U-FMR estimates. Top panel: Scenario 1. Bottom panel: Scenario 3.
